# Supplementary material for: On Limited-Memory Subsampling Strategies for Bandits
Source: arXiv:2106.10935 source file (2021-06-21)
Supplement: Supplementary file 1 [file appendix_expe.tex]

\section{Experiment}
\label{appendix:exp}

blabalbal more details on the experiments.
