# Supplementary material for: On Limited-Memory Subsampling Strategies for Bandits
Source: arXiv:2106.10935 source file (2021-06-21)
Supplement: Supplementary file 2 [file appendix_old_stuff.tex]

\section{Algorithm}

Pour l'instant on state l'algo avec forced exploration et sans la structure de round.

\begin{algorithm}
\caption{SW-LBSDA}
\label{alg:subsampling_SW}
  \begin{algorithmic}
    \STATE{ \bfseries Input.} $K$ arms, horizon $T$, sliding window length $\tau$, $B(\tau)$
    forced exploration rate
    \STATE {\bfseries Initialization.}
    $t \leftarrow 1$, $r=1$ $\forall k \in \{1, ..., K \}, N_k \leftarrow 0, N_{k,\tau} \leftarrow 0$
    \WHILE{$t < T$}
    \STATE $\mathcal{A} \leftarrow \{\}$,
    $l \leftarrow \text{leader}(N, \tau, t)$ %\mathcal{H})$
    \IF{$r=1$}
    \STATE $\cA \leftarrow \{1, \dots, K\}$ (Draw each arm once)
    \ELSE
    \FOR{$k \neq l \in 1,...,K$}
	\IF{$N_{k, \tau} \leq B(\tau)$ \OR $\bar Y_{N_k- N_{k, \tau}: N_k} > \bar Y_{N_l- N_{k, \tau}: N_l}$   }	    	\STATE $\mathcal{A} \leftarrow \mathcal{A} \cup \{ k \}$
	\ENDIF

    	\IF{$| \mathcal{A} | = 0$}
    	\STATE $\mathcal{A} \leftarrow \{l \}$
    	\ENDIF
    \ENDFOR
    \ENDIF
    \IF{ $|\mathcal{A}| > 1$}
    \STATE $a \leftarrow \text{random}(\mathcal{A})$ \;\;(random element in $\mathcal{A}$)
	\ELSE
	\STATE $a \leftarrow \mathcal{A}$
    \ENDIF
    \STATE Pull arm $a$, observe reward $Y_{a,N_a +1}$, $N_a \leftarrow N_a + 1$.
    %$\mathcal{H}_a \leftarrow \mathcal{H}_a \cup \{Y_{a, N_a} \} $
    \FOR{$ k = 1,...,K$}
    \STATE Update $N_{k, \tau}$, $t \leftarrow t+1$
    \ENDFOR
    \ENDWHILE
  \end{algorithmic}
\end{algorithm}


\section{First thoughts for the analysis with the variation budget}

We will an additional assumption for simplifying the proofs.

\begin{assumption}
We assume that the rewards are of the form
$$
r(r) = \mu_{A_r}(r) + \epsilon_r
$$
\end{assumption}

The objective in this section is to explain how the usual concentration is obtained.
The previous assumption is a bit restrictive (even more for a non-parametric analysis) but this will be our start point.

We introduce:

$$
\hat{\mu}_k(r) = \frac{1}{N_k(r, \tau)} \sum_{s= r- \tau + 1}^r \ind(k \in \mathcal{A}_{s+1}) r_k(s)
$$
and
$$
\bar{\mu}_k(r) = \frac{1}{N_k(r, \tau)} \sum_{s= r- \tau + 1}^r \ind(k \in \mathcal{A}_{s+1}) \mu_k(s)
$$

We have:
\begin{align*}
| \mu_k(r) -\hat{\mu}_k(r) | &=
|\mu_k(r) -  \bar{\mu}_k(r) + \bar{\mu}_k(r) - \hat{\mu}_k(r) | \\
&\leq  \underbrace{\left| \frac{1}{N_k(r, \tau)}   \sum_{s= r- \tau + 1}^r  \ind(k \in \mathcal{A}_{s+1})
(\mu_k(r) -  \mu_k(s)  ) \right|}_{first}  +
 \underbrace{\left|  \frac{1}{N_k(r, \tau)}   \sum_{s= r- \tau + 1}^r  \ind(k \in \mathcal{A}_{s+1} )\epsilon_r  \right|}_{second}
\end{align*}

The second term is the equivalent of the term that we would have in a stationary environment. In particular, if the environment is stationary the previous difference is exactly equal to $second$.

The first term is the bias term due to the non-stationary nature of the environment. Now, our hope is to link this term to the variation budget.


\begin{align*}
first &= \left| \frac{1}{N_k(r, \tau)}   \sum_{s= r- \tau + 1}^r  \ind(k \in \mathcal{A}_{s+1})
(\mu_k(s) -  \mu_k(r)  ) \right| \\
&= \left| \frac{1}{N_k(r, \tau)}   \sum_{s= r- \tau + 1}^r  \ind(k \in \mathcal{A}_{s+1})
\sum_{p = r- \tau + 1 }^r (\mu_k(p) -  \mu_k(p+1)  ) \right| \\
&= \left| \frac{1}{N_k(r, \tau)}   \sum_{p= r- \tau + 1}^r
\sum_{s = r- \tau + 1 }^p
\ind(k \in \mathcal{A}_{s+1})
 (\mu_k(p) -  \mu_k(p+1)  ) \right| \\
 & \leq
 \sum_{p = r- \tau + 1 }^r \left| \frac{1}{N_k(r, \tau)}
\sum_{s = r- \tau + 1 }^p
\ind(k \in \mathcal{A}_{s+1})  \right|
\left| (\mu_k(p) -  \mu_k(p+1)  ) \right| \\
& \leq  \sum_{p = r- \tau + 1 }^r | \mu_k(p) - \mu_k(p+1)|
\end{align*}

Notre guess, s'éloigner de la technique de preuve pour le modèle à $K$ bras pour faire la preuve en BV et essayer de trouver les endroits où ça pourrait bloquer.
